# Supplementary material for: Pairing in high-density neutron matter including short- and long-range correlations
Source: arXiv:1502.05673 source file (2015-02-19)
Supplement: Supplementary file 1 [file Supplement.pdf]

# Pairing in high-density neutron matter including short- and long-range correlations Supplementary material

D. Ding[1], A. Rios[2], W. H. Dickhoff[1], H. Dussan[1], A. Polls[3], and S. J. Witte[1,4]
[1]*Department of Physics, Washington University, St. Louis, Missouri 63130, USA*
[2]*Department of Physics, Faculty of Engineering and Physical Sciences, University of Surrey, Guildford, Surrey GU2 7XH, United Kingdom*
[3] *Departament d'Estructura i Constituents de la Matèria and Institut de Ciènces del Cosmos, Universitat de Barcelona, Avenida Diagonal 647, E-8028 Barcelona, Spain and*
[4]*Department of Physics and Astronomy, University of California, Los Angeles, CA 90095, USA*
(Dated: February 19, 2015)

Numerical results for self-consistent Green's functions ladder calculations with microscopic nucleon-nucleon interactions have been available in the literature for the last decade [1–3]. The pairing instability, however, precludes a direct calculation within the ladder approximation and normal propagators below the critical pairing temperature, $T_c$ [4–6]. Ladder calculations probe the pseudo-gap regime [6, 7], and hence can be used as a starting point to obtain (extrapolated) zero-temperature pairing properties. Here, we describe the extrapolation procedure to determine zero-temperature normal self-energies from sets of calculated finite temperature data. The double folding needed to compute the SRC pairing gap is also extensively discussed. Finally, we include the parameters for the analytic functions that fit the pairing gaps for the $^3P_2 - ^3F_2$ channel including short-range correlations and also for additionally including long-range correlations. The functional form we utilize was taken from Ref. [8].

## I. ZERO-TEMPERATURE EXTRAPOLATION

For a given density, ladder self-energy calculations are typically performed for a set of $N_T \approx 3$ to 10 temperatures. At each temperature, the real and imaginary parts of the self energy are stored as arrays of $\approx 4000$ to 11000 single-particle energies, $\omega$, and 70 single-particle momenta, $k$. These correspond to self-consistent solutions of the problem at a given density and finite temperature, $T$. The degeneracy parameter, $\xi = \frac{T}{\epsilon_F}$, with $\epsilon_F$ the free Fermi gas Fermi energy, is a proxy for temperature in Fermi gases and is a natural extrapolation parameter in our case[1]. Zero-temperature self-energies are thus extrapolated by fitting $\Sigma(k, \omega; T)$ in a window of $\xi$ values. For a given density, we take an upper limit of $\xi \approx 1$ and a lower limit of $\xi \gtrsim 0.07$ (as long as the pairing instability does not set in). This ensures that the finite temperature data is neither thermally dominated ($\xi \gg 1$) nor insensitive to thermal effects ($\xi \ll 1$). We note that we have used an extensive grid of self-energies in a wide range of densities and temperatures, worth a total of 13 Gb of self-energy data.

For a given $k$ and $\omega$, we fit a polynomial in degeneracies, $\Sigma(k, \omega; \xi) = \sum_{l=0}^{L} a_l(k, \omega)\xi^{2l}$ . The zero-temperature self-energy is thus the $a_0(k, \omega)$ coefficient of the fit, although in principle this fit can be used to compute self-energies at arbitrary temperatures. For practical purposes, the interpolation involves only even powers, $2l$. Self-energies, particularly close to the Fermi surface, need not be soft, continuous functions of degeneracy, particularly because self-consistent numerical calculations contain numerical limitations in accuracy. A single fit thus might extrapolate quantities in an unphysical way. For this reason, we perform not only one, but a series of fits with different values of $L$, the maximum power of the polynomial. Generally, we go from $L = 1$ (corresponding to a $T^2$ dependence) to about $L = 4$, depending on the total number of temperatures available. All polynomial fits are performed by using a $\chi^2$ minimization procedure.

A major aim of the present set of extrapolations is consistency at the microscopic and macroscopic levels. With access to the $T = 0$ self-energies and spectral functions, one can compute a series of zero temperature properties. The energy per particle, $E/A$, is obtained from the energy sum-rule at zero temperature. Alternatively, the finite temperature $\Sigma$ yields a set of energies per particle which can independently be extrapolated to zero temperature using a polynomial fit[2]. A good extrapolation procedure for the self-energy should ensure consistency between the micro- and the macroscopic results. We therefore construct a quality measure that quantifies the distance between the micro- and macroscopic extrapolations of a series of pseudo data points. The measure is built from a weighted sum of the relative differences between microscopic and macroscopic determinations of density, chemical potentials, energies, kinetic energies and $Z$-factors[3]

In the numerical implementation, we extrapolate separately the imaginary and the real parts of the self-energy.

[1] The low-temperature Sommerfeld expansion is indeed an expansion around $\xi \approx 0$ [9].

[2] For simplicity, we take the same $L$ in this fit and in that of the associated self-energy.

[3] The latter is determined independently from the discontinuity of the momentum distribution at the Fermi surface and from the on-shell derivatives of self-energies.

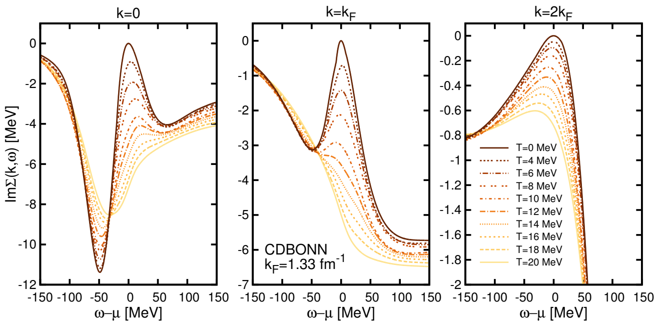


FIG. 1. Imaginary part of the self-energy around the Fermi energy at $k_F = 1.33$ fm$^{-1}$ for the CDBonn interaction. Left, centre and right panel correspond to momenta $k = 0$, $k_F$ and $2k_F$, respectively. Different lines show different temperatures, including the $T = 0$ extrapolation. Note the different vertical scales.

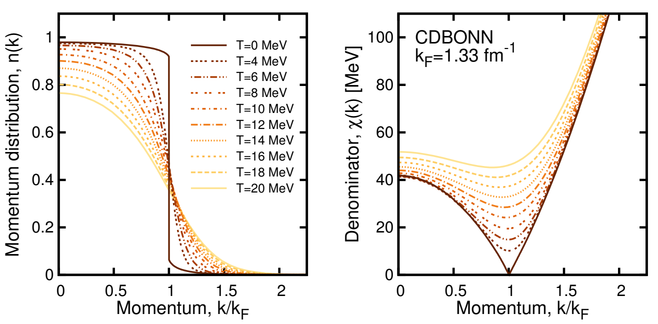


FIG. 2. Left panel: momentum distribution at $k_F = 1.33$ fm$^{-1}$ for the CDBonn interaction and different temperatures, including the $T = 0$ extrapolation. Right panel: effective single-particle denominator, $\chi(k)$, in the same conditions.

The thermodynamical consistency of the calculation is sensitive to the properties of $\Sigma$ close to the Fermi energy. This is where the temperature dependence is more difficult to capture with fits. For a given polynomial order, $L$, we therefore allow for two different options. We either take the extrapolated Im$\Sigma$ as face value[4] or we allow for a second option, where we match Im$\Sigma$ to the analytic function:

$$\mathrm{Im}\Sigma(k, \omega \approx \mu; T = 0) \approx a_k(\omega - \mu)^2 e^{-b_k(\omega-\mu)} \quad (1)$$

in the vicinity of the Fermi energy. This has the correct quadratic dependence in energy of a normal Fermi liquid [10]. The exponential factor allows for a certain degree of asymmetry below and above the Fermi surface. This function is matched to the self-energy in a given range of energies, and the new quality measure is computed. The polynomial with $L$ that minimises the quality measure, whether matched or not, is used in the extrapolation. This guarantees that the associated self-energy is consistent with both the microscopic and the macroscopic pseudo-data. The extrapolation procedure is automated at all densities, to avoid any potential biases in the calculation.

The three panels of Figure 1 show the imaginary part of the self-energy as a function of energy, $\omega$, for three characteristic momenta. Results are displayed for the charge-dependent Bonn (CDBonn) interaction [11] at $k_F = 1.33$ fm$^{-1}$, but equivalent conclusions are reached with other nucleon-nucleon (NN) interactions in this density regime. There is modest temperature dependence of Im$\Sigma$ for energies $\omega$ substantially below and above $\mu$. As the temperature decreases, however, a structure develops close to $\omega \approx \mu$, with Im$\Sigma$ becoming minimal (in absolute value). This is the area where temperature plays the most important role, and where the extrapolation procedure is most critical.

From the self-energy, one can obtain other relevant microscopic properties. The left panels of figure 2 shows, for instance, momentum distributions for the CDBonn interaction at $k_F = 1.33$ fm$^{-1}$ and a variety of temperatures. The zero-temperature momentum distribution is obtained from the extrapolated self-energy. As expected, $n(k)$ has a sharp discontinuity across the Fermi surface. The exact shape of the momentum distribution for momenta within a few percent of $k_F$ is sensitive to the extrapolation procedure. Our extrapolation procedure ensures that, on average, the discontinuity is within a few percent of the derivative of the self-energy. Below $T_c$ and as the temperature approaches zero asymptotically, the normal spectral function becomes an increasingly sharp function of energy close to the Fermi surface. It is important to keep track of these narrow structures in the calculation of $n(k)$. We therefore correct the momentum distribution by including a quasi-particle term that takes into account the missing strength, as estimated by the (missing) spectral function sum rule. We have tested this procedure against the momentum distribution obtained from derivatives of the zero-temperature self-energy [12] and have found quantitative agreement.

## II. DOUBLE ENERGY CONVOLUTION

After the zero-temperature self-energy extrapolation is performed, pairing calculations require as input the double energy convolution of Eq. (5) with the substitution $\mathcal{A}_s \to \mathcal{A}$. We first note the formal similarities of Eqs. (5) and (2). In practical terms, the experience gathered in performing this double convolution in finite temperature calculations is useful in computing the energy denominator [13]. Pairing calculations, particularly in the $^3P_2$–$^3F_2$ channel, are very sensitive to the Fermi surface region, and inaccuracies on the double folding are amplified in final gap solutions. In particular, missing strength cor-

[4] Im$\Sigma \leq 0$ is imposed throughout, though.

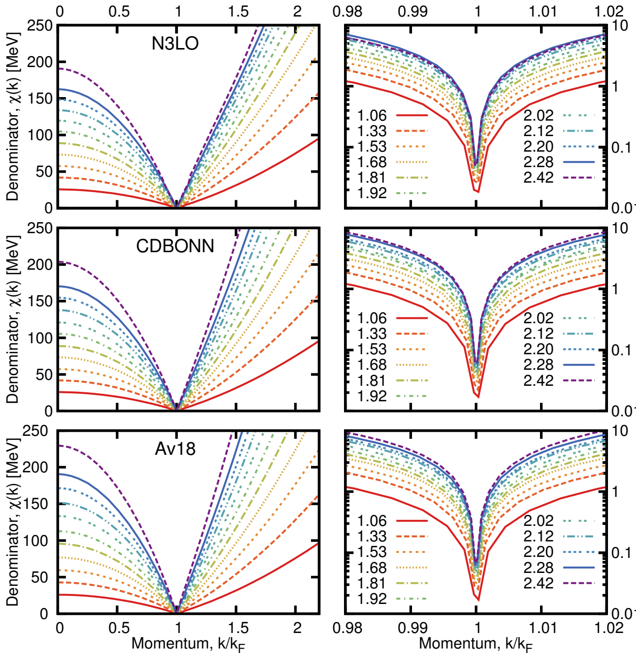


FIG. 3. Left panels: energy denominator at $T = 0$ as a function of momentum for a variety of Fermi momenta. Top, center and bottom panels correspond to the N3LO [14], CD-Bonn [11] and AV18 [15] interactions, respectively. Right panels: the same quantity around the Fermi surface in a logarithmic scale.

rections, analogous to those just discussed for $n(k)$, are important in the double convolution. We thus use the following sum-rule of the lowest-order two-particle propagator,

$$\int \frac{d\Omega}{2\pi} \mathcal{G}^0_{II}(k, k' = k, \Omega) = 1 - 2n(k)\,, \tag{2}$$

to estimate the missing strength at a given momentum, $\varsigma_k$. The missing strength correction in our ladder calculations is of the order of a few percent or less away from the Fermi surface. $\varsigma_k$ is generally largest (50 % or above) for momenta which are within $2 - 3\,\%$ of the Fermi surface. The energy denominator is corrected employing a quasi-particle approximation,

$$\frac{1}{2\widetilde{\chi}(k)} \rightarrow \frac{1}{2\widetilde{\chi}(k)} + \frac{\varsigma_k}{2(\varepsilon_k - \mu)}\,. \tag{3}$$

This yields soft, continuous functions of momentum in regions arbitrarily close to $k_F$. The right panel of Fig. 2 shows energy denominators as a function of momenta for a variety of temperatures, including the $T = 0$ extrapolated values.

The density dependence of the zero-temperature double convolution obtained with the three NN interactions considered is displayed in Fig. 3. The denominator shows a minimum around the Fermi surface, and a linear behavior around $k = k_F$. The value of $\chi(k)$ at $k = k_F$ is relatively small, but non-zero. The right panels provide a more detailed view of the density dependence of $\chi(k)$ around $k_F$ employing a logarithmic scale. Without missing strength corrections, the near-Fermi-surface behavior would be erratic. The missing-strength-corrected calculation, in contrast, provides a well-defined function of momentum and density. We note that the different NN interactions enter the denominator calculation via the convolution of different spectral functions. The integrated convolution smears out the differences between NN potentials, and hence the results obtained for $\chi(k)$ (and its density dependence) are relatively similar for all three interactions.

## III. PARAMETERS FOR FITS TO CALCULATED GAPS

A convenient parametrization of the gap function is given by

$$\Delta(k_F) = \Delta_0 \frac{(k_F - k_0)^2}{(k_F - k_0)^2 + k_1} \frac{(k_F - k_2)^2}{(k_F - k_2)^2 + k_3}\,, \tag{4}$$

with $\Delta_0, k_0, k_1, k_2$, and $k_3$ parameters as *e.g.* utilized in Ref. [8] . We include in Table I the values of these parameters for the fits shown in Fig. 2 of the paper for the different interactions.

TABLE I. Parameters generated by a fit to the calculated gaps for the AV18, CDBonn, and N3LO interaction in the $^3P_2 -^3 F_2$ channel. The first line contains the results for the inclusion of SRC and the second also the effect of LRC for each interaction.

| | $\Delta_0$ [MeV] | $k_0$ fm$^{-1}$ | $k_1$ fm$^{-2}$ | $k_2$ fm$^{-1}$ | $k_3$ fm$^{-2}$ |
|---|---|---|---|---|---|
| AV18 SRC | 0.064 | 1.058 | 0.26 | 1.98 | 0.0032 |
| SRC+P | 0.23 | 1.058 | 0.605 | 2.19 | 0.069 |
| CDB SRC | 0.15 | 1.058 | 0.49 | 2.28 | 0.12 |
| SRC+P | 0.37 | 1.041 | 0.49 | 2.803 | 0.87 |
| N3LO SRC | 0.49 | 1.058 | 1.34 | 2.58 | 0.4 |
| SRC+P | 0.37 | 1.058 | 0.51 | 2.77 | 0.22 |


[1] T. Frick and H. Müther, Phys. Rev. C **68**, 034310 (2003).
[2] A. Rios, *Thermodynamical Properties of Nuclear Matter from a Self-Consistent Green's Function Approach,*, Ph.D. thesis, University of Barcelona (2007).
[3] V. Somà and P. Bożek, Phys. Rev. C **78**, 054003 (2008).

[4] A. Ramos, *Beyond a Mean Field Description of Nuclear Systems within Self-Consistent Green Functions Theory*, Ph.D. thesis, University of Barcelona (1988).

[5] T. Alm, B. Friman, G. Röpke, and H. Schulz, Nucl. Phys. A **551**, 45 (1993).

[6] H. Müther and W. H. Dickhoff, Phys. Rev. C **72**, 054313 (2005).

[7] A. Schnell, G. Röpke, and P. Schuck, Phys. Rev. Lett. **83**, 1926 (1999).

[8] W. C. G. Ho, K. G. Elshamouty, C. O. Heinke, and A. Y. Potekhin, Phys. Rev. C **91**, 015806 (2015).

[9] N. W. Ashcroft and N. D. Mermin, *Solid State Physics*, edited by F. Seitz and D. Turnbull (Brooks Cole, 1976) p. 848.

[10] J. M. Luttinger, Phys. Rev. **121**, 942 (1961).

[11] R. Machleidt, F. Sammarruca, and Y. Song, Phys. Rev. C **53**, R1483 (1996).

[12] A. Rios, A. Polls, and W. H. Dickhoff, Phys. Rev. C **79**, 064308 (2009).

[13] T. Frick, *Self-consistent Green's Functions in Nuclear Matter at Finite Temperature*, Ph.D. thesis, University of Tübingen (2004).

[14] D. R. Entem and R. Machleidt, Phys. Rev. C **68**, 041001 (2003).

[15] R. B. Wiringa, V. G. J. Stoks, and R. Schiavilla, Phys. Rev. C **51**, 38 (1995).
